# Supplementary material for: Towards Learning-Augmented Peer-to-Peer Networks: Self-Stabilizing Graph Linearization with Untrusted Advice
Source: arXiv:2504.02448 source file (2025-04-03)
Supplement: Supplementary file 1 [file Tables.tex]

\section{Helpful Tables}

\begin{table}[!htp]
\begin{center}
    \begin{tabular}{|l|c|c|}
    \hline
     Variable & Store ids? \\%& Brief description\\
    \hline
    $u.L$ & \cmark \\%& \\
    $u.R$ & \cmark \\%& \\
    $u.\mathit{vID}$ & \xmark \\%& \\
    $u.\mathit{flyID}$ & \cmark \\%& \\
    \hdashline
    $u.\text{\emph{c-par}}$ & \xmark \\%& \\
    $u.\text{\emph{c-dist}}$ & \xmark \\%& \\
    $u.\text{\emph{c-ids}}$ & \cmark \\%& \\
    \hdashline
    $u.\mathit{exit}$ & \xmark \\%& \\
    \hline
    \end{tabular}
    \caption{Flyover variables.}
    \label{tab:fly-vars}
\end{center}
\end{table}

\begin{table}
\begin{center}
    \begin{tabular}{|l|c|c|}
    \hline
     Variable & Store ids? \\%& Brief description\\
    \hline
    $u.t$ & \xmark \\%& \\
    $u.\mathit{dist}$ & \xmark \\%& \\
    \hline
    \end{tabular}
    \caption{Advice variables.}
    \label{tab:adv-vars}
\end{center}
\end{table}
